# Supplementary material for: Pair potential with submillikelvin uncertainties and nonadiabatic treatment of the halo state of helium dimer
Source: arXiv:1706.05687 ancillary file (2017-08-04)
Supplement: Supplementary file 1 [file supplemental.pdf]

# Supplemental information for: "Pair potential with submillikelvin uncertainties and nonadiabatic treatment of the halo state of helium dimer"

Michał Przybytek,[1,*] Wojciech Cencek,[2] Bogumił Jeziorski,[1] and Krzysztof Szalewicz[2]
[1] *Department of Chemistry, University of Warsaw, Pasteura 1, 02-093 Warsaw, Poland*
[2] *Department of Physics and Astronomy, University of Delaware, Newark, DE 19716, USA*
(Dated: July 24, 2017)

Supplemental information consists of 6 files:

| | |
|---|---|
| `supplemental.pdf` | this file, |
| `S1_BO.txt` | interaction energy at the Born-Oppenheimer level, |
| `S2_postBO.txt` | post-BO (adiabatic, relativistic, and QED) corrections to the interaction energy, |
| `S3_NAPT.txt` | diagonal nonadiabatic correction to the interaction potential and corrections to the $R$-dependent rotational and vibrational masses, |
| `S4_basis_sets.txt` | composition of the orbital basis sets d$X$Zcp and d$X$Z+$n$p. |
| `S5_potentials.f90` | Fortran code with analytic functions fitted to calculated data points, |

### File S1_BO.txt

The file contains the complete set of 46 interaction energies of the helium dimer, $V_{\rm BO}$ (in kelvin, 1 hartree = 315775.13 K), computed at the Born-Oppenheimer (BO) level for distances $1.0 \leq R \leq 9.0$ bohr using four-electron ECG expansions. The entries in the second column, $V_{\rm ub}$, are strict upper bounds, obtained by subtracting the exact helium monomer energies from the variational dimer energies in the largest (6788 term) basis set. The entries in the third column are interaction energies extrapolated to the complete basis set (CBS) limit, as described in the main paper. Their uncertainties are given in the fourth column.

For completeness, there are also included two symmetry-adapted perturbation theory (SAPT) interaction energies from Ref. [1] (for $R = 10.0$ and 12.0 bohr) which were used to construct the analytic fit of the BO interaction energies.

### File S2_postBO.txt

The file contains recommended values (in kelvin, 1 hartree = 315775.13 K) and estimated uncertainties of the adiabatic, $V_{\rm ad}$, relativistic, $V_{\rm rel}$, and QED, $V_{\rm QED}$, corrections to interaction energy of the helium dimer. In computations we assumed mass of the helium atom nucleus $m_n = 7294.29954136\, m_e$ and fine structure constant $\alpha = 1/137.035999139$. $V_{\rm ad}$ and $V_{\rm rel}$ are given for a set of 55 interatomic distances $1.0 \leq R \leq 30.0$ bohr, and $V_{\rm QED}$ is given for a set of 17 distances $1.0 \leq R \leq 12.0$ bohr. The file contains also our recommended values and estimated uncertainties of individual components $V_{\rm CG}$, $V_{\rm D1}$, $V_{\rm D2}$, and $V_{\rm Br}$ of $V_{\rm rel}$

$$V_{\rm rel}(R) = V_{\rm CG}(R) + V_{\rm D2}(R) + V_{\rm Br}(R), \qquad \text{[see Eq. (53) of Ref. [2]]}, \tag{1}$$

and $V_{\rm QED}$

$$V_{\rm QED}(R) = 0.037\,807\,203\, V_{\rm D1}(R) - 0.027\,938\,416\, V_{\rm D2}(R) + V_{\rm AS}(R), \qquad \text{[see Eq. (54) of Ref. [2]]}, \tag{2}$$

defined in detail in Ref. [2]. The Araki-Sucher, $V_{\rm AS}$, component was taken from Ref. [2] and is not reported here.

### File S3_NAPT.txt

The file contains recommended values (in atomic units, multiplied by $\mu_n^2$, where $\mu_n$ is the reduced mass of the nuclei) of the functions appearing in the effective radial Schrödinger of the nonadiabatic perturbation theory (NAPT): the diagonal nonadiabatic correction to the interaction potential of the helium dimer, $\mu_n^2 V_{\rm na}^{\rm int}$, and $R$-dependent rotational, $\mu_n^2 \mathcal{W}_{\perp}^{\rm int}$, and vibrational, $\mu_n^2 \mathcal{W}_{\parallel}^{\rm int}$, mass corrections. The values are provided for a set of 52 interatomic distances $1.0 \leq R \leq 18.0$ bohr.

### File S4_basis_sets.txt

The orbital basis sets d$X$Zcp and d$X$Z+$n$p can be reconstructed using data from two files

**A:** file `S1_Basis_sets.txt` from supplementary information for Ref. [2],
**B:** file `S4_basis_sets.txt`.

To produce d$X$Zcp basis set, $X = 3, \ldots, 8$, one needs to combine:

1. contracted $s$ function from SECTION I.a of **A**,
2. uncontracted $s$ functions from an appropriate column from SECTION I.b of **A**,
3. contracted $p$ function from SECTION IV of **B**,
4. uncontracted $p$, $d$, $f, \ldots$ functions from an appropriate column from SECTION III of **A**.

To produce d$X$Z+$n$p basis set, $X = 3, \ldots, 8$, $n = 1, \ldots, 5$ one needs to combine:

1. uncontracted $s$ functions from SECTION II of **A**,
2. uncontracted $p$ functions form an appropriate column and row from SECTION V of **B**,
3. uncontracted $p$, $d$, $f, \ldots$ functions from an appropriate column from SECTION III of **A**.

### File S5_potentials.f90

The file contains code of the Fortran90 module `potentials` that provides 14 functions:

| | |
|---|---|
| `V_BO(R)` | fit to the Born-Oppenheimer interaction energy $V_{\rm BO}$, |
| `V_AD(R)` | fit to the adiabatic correction potential $V_{\rm ad}$, |
| `V_REL(R)` | fit to the relativistic correction potential $V_{\rm rel}$, |
| `V_QED(R)` | fit to the QED correction potential $V_{\rm QED}$, |
| `V(R,ret)` | sum of the fits to $V_{\rm BO}$, $V_{\rm ad}$, $V_{\rm rel}$, and $V_{\rm QED}$, |
| `mu2V_NA(R)` | fit to the diagonal nonadiabatic correction $\mu_n^2 V_{\rm na}^{\rm int}$, |
| `mu2Wr(R)` | fit to the rotational mass correction $\mu_n^2 \mathcal{W}_\perp^{\rm int}$, |
| `mu2Wv(R)` | fit to the vibrational mass correction $\mu_n^2 \mathcal{W}_\parallel^{\rm int}$, |
| `diff_mu2Wv(R)` | first derivative of the fit to $\mu_n^2 \mathcal{W}_\parallel^{\rm int}$, |
| `sigma_BO(R)` | fit to the uncertainties of the Born-Oppenheimer energy $\sigma_{\rm BO}$, |
| `sigma_AD(R)` | fit to the uncertainties of the adiabatic correction $\sigma_{\rm ad}$, |
| `sigma_REL(R)` | fit to the uncertainties of the relativistic correction $\sigma_{\rm rel}$, |
| `sigma_QED(R)` | fit to the uncertainties of the QED correction $\sigma_{\rm QED}$, |
| `sigma(R)` | square root of the sum of squares of fits to $\sigma_{\rm BO}$, $\sigma_{\rm ad}$, $\sigma_{\rm rel}$, and $\sigma_{\rm QED}$. |

INPUT:

| | | |
|---|---|---|
| `R` | double precision | distance in bohr, |
| `ret` | logical, optional | should the retardation be switched on (`.true.`) or not (`.false.`); if not present the value `.false.` is assumed. |

OUTPUT:

double precision value of a given potential or error estimation in atomic units.

EXAMPLE:

```
use potentials
write(*,*) V(5.6d0),V(5.6d0,.true.),sigma(5.6d0)
end
```

gives the result: `-3.4820829862439775E-005 -3.4820451375400200E-005 7.9823127926846210E-010`

*Notes:*

1. Analytic functions used to fit the computed values of $V_{\rm BO}(R)$, $V_{\rm ad}(R)$, $V_{\rm rel}(R)$, $V_{\rm QED}(R)$, $\mu_n^2 V_{\rm na}^{\rm int}(R)$, $\mu_n^2 \mathcal{W}_\perp^{\rm int}(R)$, and $\mu_n^2 \mathcal{W}_\perp^{\rm int}(R)$ have the same general form
$$\sum_{k=1}^{M} e^{-a_k R} \sum_{i=I_0}^{I_1} P_{ik} R^i - \sum_{n=N_0}^{N_1} f_n(\zeta R) \frac{C_n}{R^n}, \tag{3}$$
where $f_n(x) = 1 - e^{-x} \sum_{i=0}^{n} x^i/i!$ is the Tang-Toennies damping function. The summation limits $M$, $I_0$, $I_1$, $N_0$, $N_1$ are listed in the main text and in the file `S5_potentials.f90`. The values of the parameters $a_k$, $P_{ik}$, $\zeta$, and $C_n$ (in atomic units) can be found in the file `S5_potentials.f90`.

In fitting of $V_{\rm BO}(R)$, the linear parameters $P_{ik}$ were constrained by imposing the condition $V_{\rm BO}(R) = 4/R + (E_{\rm Be} - 2E_{\rm He}) + \mathcal{O}(R^2)$ assuring the right short-range asymptotics of the potential. The known accurate ground-state energies of the beryllium and helium atoms, $E_{\rm Be} = -14.667356498$ hartree [3] and $E_{\rm He} = -2.903724377$ hartree [4], were used. The long-range asymptotic constants of $V_{\rm BO}(R)$ were fixed at the same values as in Ref. [2]. Only $C_{11}$ and $C_{13}$ were replaced by more accurate values from Ref. [5].

In the least-squares fitting of $V_{\rm BO}(R)$, $V_{\rm ad}(R)$, $V_{\rm rel}(R)$, and $V_{\rm QED}(R)$ we used the inverse squares of the corresponding uncertainties as the weighting factors. The quality of the fits is shown in Table I. In the least-squares fitting of $\mu_n^2 V_{\rm na}^{\rm int}(R)$, $\mu_n^2 \mathcal{W}_{\perp}^{\rm int}(R)$, and $\mu_n^2 \mathcal{W}_{\perp}^{\rm int}(R)$ as the weighting factors we used the inverse squares of values of these functions multiplied by 0.05.

TABLE I. Maximum and average ratios of the fit errors to the data point uncertainties for the fits of the Born-Oppenheimer interaction energy and adiabatic, relativistic, and QED corrections

| potential | Max(fit error/$\sigma$) | Average(fit error/$\sigma$) |
|---|---|---|
| $V_{\rm BO}$ | 0.92 | 0.16 |
| $V_{\rm ad}$ | 0.64 | 0.16 |
| $V_{\rm rel}$ | 0.74 | 0.24 |
| $V_{\rm QED}$ | 0.68 | 0.14 |

2. To check if the number of data points used was sufficient to obtain an accurate fit of $V_{\rm BO}(R)$ in the whole range of $R$, we performed the following test. For each of the 48 data points $R_i$ we generated a separate fit of the form of Eq. (3) using the data set with this point removed. In this process only linear parameters $P_{ik}$ were fitted, while the nonlinear parameters $a_k$ and $\zeta$ were taken from the final fit. Then, for each of these new 48 fits, we compared the interaction energy predicted at the removed point with the *ab initio* value. The only instance where the predicted and *ab initio* energies deviated by more than $1\sigma$ was at the distance $R = 2.0$ bohr. But even then, the deviation was marginal, *i.e.*, only $1.006\sigma$. Since this distance corresponds to the high-energy area on the repulsive wall ($3.6 \times 10^4$ K), this behavior is inconsequential. Let us note that a similar test, with both linear and nonlinear parameters optimized, was first performed for the initial set of 16 data points, and it revealed that this number of points is insufficient and had to be enlarged. In Ref. [2], an analogous test, see Sect. VI.F of Ref. [2], confirmed that the 18 points used in Ref. [2] were sufficient (because of the larger uncertainties of calculations than those of the present work).

3. Analytic functions used to represent the estimated uncertainties of $V_{\rm BO}(R)$, $V_{\rm ad}(R)$, $V_{\rm rel}(R)$, and $V_{\rm QED}(R)$ have the general form

$$\sigma_X(R) = s_0^X e^{-a_0^X R} + \sum_{i=1}^{n_X} s_i^X e^{-a_i^X R^2}, \quad X = \text{BO, ad, rel, QED} \tag{4}$$

(the estimated uncertainties are listed in the fourth column in the file `S1_BO.txt` and in the third column in the file `S2_postBO.txt`). The summation limits $n_X$ in Eq. (4) are listed in the main text and in the file `S5_potentials.f90`. The values of the parameters $a_i^X$ and $s_i^X$, $i = 0, \ldots, n_X$, (in atomic units) can be found in the file `S5_potentials.f90`. At the BO level the largest distance considered by us is $R = 9$ bohr, whereas the points $R = 10$ and 12 bohr are taken from Ref. [1]. Since the large-$R$ behaviour of the uncertainties is essentially determined by these two points, we fixed the large-$R$ decay of $\sigma_{\rm BO}(R)$ by setting the exponent $a_0^{\rm BO}$ to the value 0.8074 taken from Ref. [1] (denoted there as $D_\sigma$). The same value was used for $a_0^{\rm QED}$. In the case of the remaining functions, when data are available up to $R = 30$ bohr, all the parameters were fitted.

Our $\sigma_{\rm X}(R)$ are intended to follow general trends in the $R$-dependence of the estimated uncertainties (not including the fits errors which will be accounted for later on) and to bound *most* values from above. This is a departure from the previous work of our group where the upperbounding property was strictly imposed. With the current, significantly reduced values of uncertainties and with two types of values in the BO component (fully optimized and only linearly optimized, see main text), the variation of uncertainties with $R$ is so irregular that imposing the strict constraint would make $\sigma_X(R)$ to overestimate the uncertainties at a large number of points. For the same reason, we had to discard the uncertainties with the values significantly smaller than the neighboring ones. With these assumptions, the fit of uncertainties was performed using the standard least-square method. The results are shown in Fig. 1. As one can see, despite our assumptions, the curve $\sigma_{\rm BO}(R)$ does

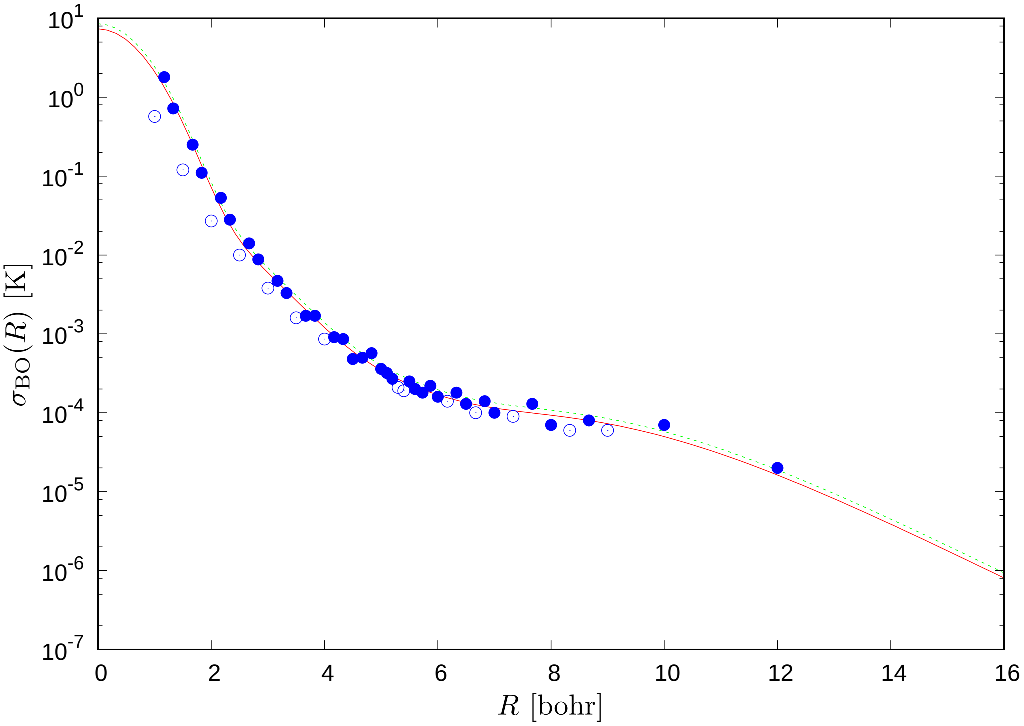


FIG. 1. Estimated uncertainties (full and open dots) of the Born-Oppenheimer potential $V_{\rm BO}$ and the analytic function $\sigma_{\rm BO}(R)$ of the form (4) used to represent the data. Red solid line is the least-square fit to points shown as full dots, and green dashed line is the same curve multiplied by $(1 + \delta^{\rm BO}) = 1.16$ (see text). Note logarithmic scale on the vertical axis.

bound most uncertainties from above. This function is below the estimated uncertainties (at most by $0.28\sigma$) for eighteen distances for which the nonlinear parameters of the ECG basis set were not fully optimized. Thus, our fit of uncertainties is an upper bound for the fully optimized energies.

To account for the fitting errors of the corresponding potentials, the fitted functions were multiplied by $(1+\delta^X)$, where $\delta^X$ is the average ratio of the potential fit error to the estimated uncertainty at each $R$ (listed in the third column of Table I). The final $\sigma_{\rm X}(R)$ in the file `S5_potentials.f90` include this factor.

* mitek@tiger.chem.uw.edu.pl


[1] M. Jeziorska, W. Cencek, K. Patkowski, B. Jeziorski, and K. Szalewicz, J. Chem. Phys. **127**, 124303 (2007).
[2] W. Cencek, M. Przybytek, J. Komasa, J. B. Mehl, B. Jeziorski, and K. Szalewicz, J. Chem. Phys. **136**, 224303 (2012).
[3] M. Puchalski, J. Komasa, and K. Pachucki, Phys. Rev. A **87**, 030502(R) (2013).
[4] H. Nakashima and H. Nakatsuji, J. Chem. Phys. **128**, 154107 (2008).
[5] L. Y. Tang, Z. C. Yan, T. Y. Shi, and J. Mitroy, Phys. Rev. A **84**, 052502 (2011).
